# Supplementary material for: Relaxing Accurate Initialization Constraint for 3D Gaussian Splatting
Source: arXiv:2403.09413 source file (2024-05-28)
Supplement: Supplementary file 2 [file computation_table_memory.tex]

\begin {table}[!hbt]
    \caption{\textbf{Memory size}\tablefootnote{Except for 3DGS(DSV) and Ours, we copied the memory size of different models from 3DGS~\cite{kerbl20233d}.}}
    \centering
    \resizebox{0.6\textwidth}{!}{
    \begin{tabular}{c|c|c|c}
        \toprule & Mip-NeRF360 &  Tanks\&Temples & Deep Blending \\
        \midrule 
        
        Plenoxels  & 2.1GB & 2.3GB & 2.7GB \\

        INGP-Base  & 13MB & 13MB & 13MB  \\

        INGP-Big & 48MB & 48MB & 48MB \\

        3DGS & 734MB & 411MB & 676MB \\

        3DGS (DSV) & 592MB & 365MB & 582MB \\
        \hlrow Ours & 581MB & 359MB & 545MB \\

    \end{tabular}
    }

    \label{exp:memory_size}
\end{table}
