# Supplementary material for: Relaxing Accurate Initialization Constraint for 3D Gaussian Splatting
Source: arXiv:2403.09413 source file (2024-05-28)
Supplement: Supplementary file 3 [file movement.tex]

\begin {table}[!hbt]
    \caption{\textbf{Analysis of points movement}}
    \centering
    \resizebox{0.8\textwidth}{!}{
    \begin{tabular}{l|c|c|c}
        \toprule  & 3DGS (SfM) & 3DGS (Random) & Ours (Random) \\
        \midrule
        
        Means  & 0.349 &  0.184& 12.100\\

        Stds of movement & 0.726& 0.297& 18.600\\

        Top 1\% & 3.418& 1.524& 82.721\\
        Top 5\% & 1.444& 0.714& 35.486\\
        Top 10\% & 0.898& 0.458& 24.866\\
        \bottomrule
    \end{tabular}
    }

    \label{tab:movement}
\end{table}
